# Supplementary material for: Measuring the locations and properties of VHF sources emitted from an aircraft flying through high clouds
Source: arXiv:2509.16574 source file (2025-09-20)
Supplement: Supplementary file 1 [file AirPlane-SI.pdf]

# Measuring the locations and properties of VHF sources emitted from an aircraft flying through high clouds

Olaf Scholten<sup>1,2\*</sup>, Marten Lourens<sup>1,2</sup>, Stijn Buitink<sup>3</sup>,  
Steve Cummer<sup>4</sup>, Joe Dwyer<sup>5</sup>, Brian M. Hare<sup>1,2</sup>, Tim Huege<sup>6</sup>,  
Ningyu Liu<sup>5</sup>, Katie Mulrey<sup>7</sup>, Anna Nelles<sup>8,9</sup>, Chris Sterpka<sup>2</sup>,  
T. N. Gia Trinh<sup>10</sup>, Paulina Turekova<sup>1,2</sup>, Sander ter Veen<sup>2</sup>

<sup>1</sup>Kapteyn Astronomical Institute, University of Groningen, P.O. Box 72,  
9700 AB Groningen, Netherlands.

<sup>2</sup>Netherlands Institute for Radio Astronomy (ASTRON), Dwingeloo,  
The Netherlands.

<sup>3</sup>Interuniversity Institute for High-Energy, Vrije Universiteit Brussel,  
Pleinlaan 2, 1050 Brussels, Belgium.

<sup>4</sup>Department of Electrical and Computer Engineering, Duke University,  
Durham, NC, 27708, USA.

<sup>5</sup>Department of Physics & Astronomy and Space Science Center (EOS),  
University of New Hampshire, Durham NH 03824 USA.

<sup>6</sup>KIT, Karlsruhe, Germany.

<sup>7</sup>Department of Astrophysics/IMAPP, Radboud University Nijmegen,  
Nijmegen, The Netherlands.

<sup>8</sup>Deutsches Elektronen-Synchrotron DESY, Platanenallee 6, 15738  
Zeuthen, Germany.

<sup>9</sup>Erlangen Centre for Astroparticle Physics (ECAP),  
Friedrich-Alexander-Universität Erlangen-Nürnberg, 91058 Erlangen,  
Germany.

<sup>10</sup>Physics Education Department, School of Education, Can Tho  
University, Campus II, 3/2 Street, Ninh Kieu District, Can Tho City,  
Viet Nam.

\*Corresponding author(s). E-mail(s): [o.scholten@rug.nl](mailto:o.scholten@rug.nl);

## Abstract

We show that it is possible to locate the few places on the body of an airplane, while it is flying through high clouds, from which broad-band, pulsed, radiation is emitted at Very High Frequency (VHF) radio frequencies. This serendipitous find was made whilst imaging a lightning flash using the Low-Frequency Array (LOFAR). This observation provides insights into the way the airplane sheds the electrical charge it acquires when flying through clouds. Furthermore, this observation allowed us to test and improve the precision and accuracy for our lightning observation techniques.

Our findings indicate that with the improved procedure the location precision for strong pulses is better than 50 cm, with the orientation of linear polarization being accurate to within  $25^\circ$ . For the present case of a Boeing 777-300ER, VHF emissions were observed exclusively associated with the two engines, as well as a specific spot on the tail. Despite the aircraft flying through clouds at an altitude of 8 km, we did not detect any emissions from electrostatic wicks.

**Keywords:** Beamforming; interferometry; static charge; VHF emission from airplane

## 1 Supplementary Information

We show here the data from a preliminary analysis of the data on a plane observed in the flash named 20A-8, recorded by LOFAR on August 14, 2020 at 14:32:41 UTC. Like the Plane discussed in the main paper, this particular one was also found serendipitously when looking in detail of some particular features in the lightning flash. The intensity of the sources on this plane, and Airbus 318-100, were much weaker than the brightest sources on the plane discussed in the main paper, which is the reason that it was not seen in initial scans of the images. The LOFAR-coordinates (centered at the LOFAR core) of this plane are (N,E,h)=(4.09, -2.815, 11.662) km implying that it is flying almost overhead to the core. Also this plane was flying through high clouds that were reaching altitudes of over 13 km.

For the exploratory analysis shown in Fig. 1 we have explored a relatively short section of data (30 ms) at a time there was no lightning activity seen in this LOFAR recording. We used the ATRI-D imager as discussed in the main part of this work where we have relaxed the constraints on the quality of fit and show all sources in this time span with  $Q < 1.2$ . Like is the case for the main paper the sources are concentrated at the tail of the plane and near the engines. The intensity of the engine events is comparable to those shown in the main paper. The intensity of the sources at the tail are, for this case, of similar magnitude as the engine sources, in stark contrast with the case shown in the main paper.

The Data on the polarization directions of the sources show basically the same features as the case of the main paper where the polarization direction of the sources at the tail have a distinctly different orientation as those associated with the engines. The polarization direction of the tail sources appears to be essentially perpendicular to the airplane surface, like is the case in the main part of the paper.

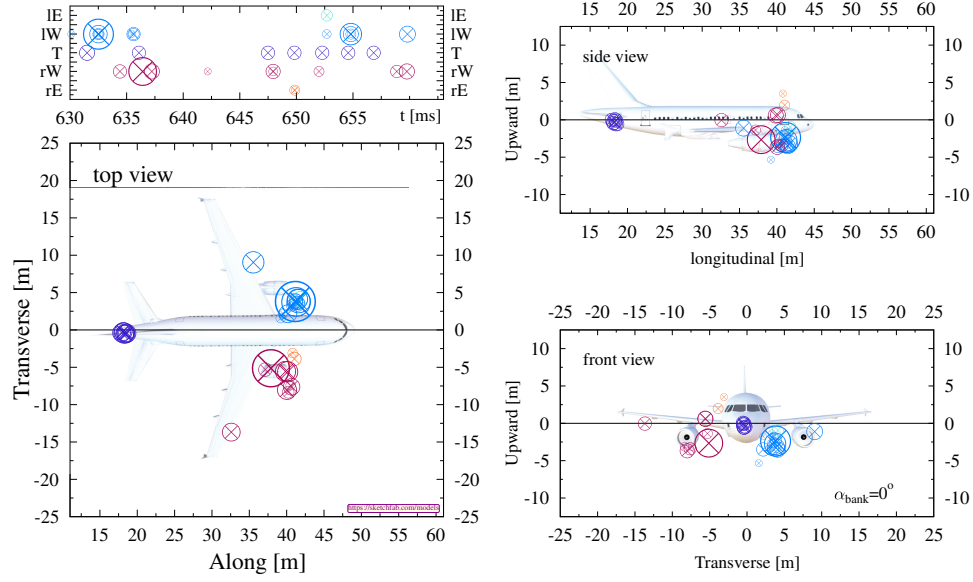

**SI Figure 1:** The imaged VHF-sources transformed into a frame that is co-moving with the plane in flash 20A-8. The ‘Along’-axis is pointing in the flight direction of the plane. The size of the wagon wheels indicates intensity of each source. The color coding of the events is following the position on the airplane where ‘rEa’, ‘rEb’, ‘T’, ‘lEb’, ‘lEa’ label right engine front, right engine back, tail, left engine back, and left engine front respectively. The image of the airplane, a Airbus-318-100 is taken from [Sketchfab](#).

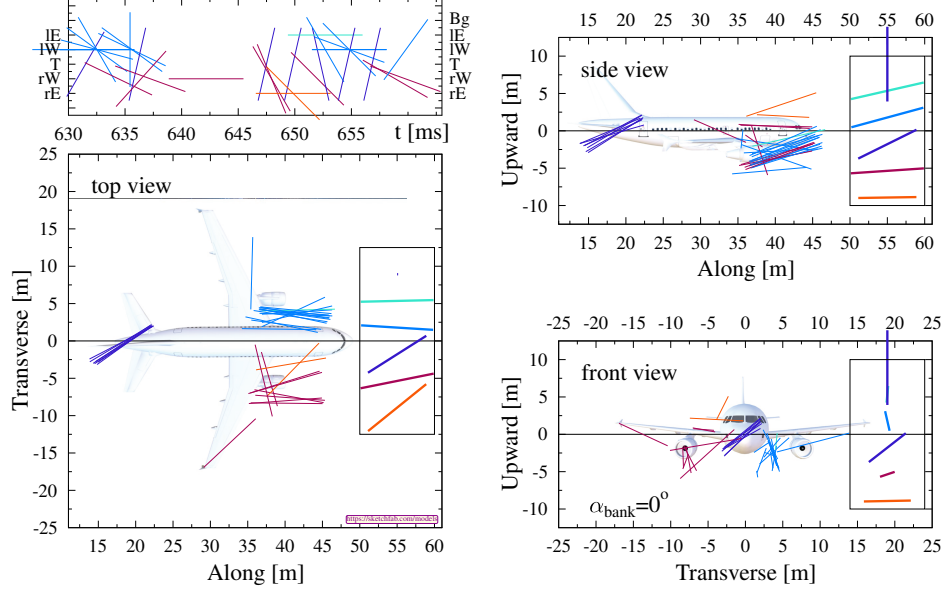

**SI Figure 2:** The analysis of the main linear polarization direction of each source as determined through the principal component analysis. The widths of the bars is proportional to the square root of the strength of the principal linear polarization component for all panels. In the top left panel the length of the bars indicate the fraction of linear polarization. In the bottom left panel and right panels show the projection of the (normalized) 3-D polarization orientation of each source on different planes that are aligned with the airplane. The inset on the right of each panel shows the same for the average of the events (width of the bar is constant).
